# Supplementary material for: Deficit of primitive compositions in binary asteroids and pairs
Source: arXiv:2302.02668 source file (2023-02-06)
Supplement: Supplementary file 1 [file binp_cits.tex]

\begin{tabular}{llrrrrrrrrrr}
	\toprule
	Number & Name & D & $\sigma_D$ & D Ref. & $p_V$ & $\sigma_{p_V}$ & Tax. method & Tax. scheme & Class & Waverange & Tax. Ref. \\
	\midrule
\hline \\2602 & Moore & - & - & - & - & - & Phot & Bus-DeMeo & S & VIS & {\cite{2013Icar..226..723D}} \\
2883 & Barabashov & 4.96 & 0.07 & {\cite{2014ApJ...791..121M}} &  0.32 & 0.19  & Phot & Bus-DeMeo & S & VIS & {\cite{2013Icar..226..723D}} \\
5500 & Twilley & 4.26 & 0.11 & {\cite{2022PSJ.....3...30M}} &  0.3 & 0.19  & Phot & Bus-DeMeo & S & VIS & {\cite{2013Icar..226..723D}} \\
6245 & Ikufumi & 7.88 & 0.21 & {\cite{2016AJ....152...63N}} &  0.13 & 0.19  & Phot & Bus-DeMeo & X & VIS & {\cite{2021A&A...652A..59S}} \\
7393 & Luginbuhl & 5.43 & 0.1 & {\cite{2015ApJ...814..117N}} &  0.27 & 0.19  & Phot & Bus-DeMeo & S & NIR & {\cite{2018A&A...617A..12P}} \\
9474 & Cassadrury & 3.57 & 0.16 & {\cite{2011ApJ...741...68M}} &  0.24 & 0.21  & Phot & Bus-DeMeo & S & VIS & {\cite{2013Icar..226..723D}} \\
18303 & 1980 PU & - & - & - & - & - & Phot & Bus-DeMeo & S & VIS & {\cite{2022A&A...658A.109S}} \\
20882 & Paulsanchez & - & - & - & - & - & Phot & Bus-DeMeo & S & VIS & {\cite{2013Icar..226..723D}} \\
25021 & Nischaykumar & 2.15 & 0.52 & {\cite{2011ApJ...741...68M}} &  0.16 & 0.52  & Phot & Bus-DeMeo & L & VIS & {\cite{2022A&A...658A.109S}} \\
26420 & 1999 XL103 & - & - & - & - & - & Phot & Bus-DeMeo & V & VIS & {\cite{2021A&A...652A..59S}} \\
72036 & 2000 XM44 & 3.1 & 0.58 & {\cite{2016AJ....152...63N}} &  0.28 & 0.42  & Phot & Bus-DeMeo & S & VIS & {\cite{2022A&A...658A.109S}} \\
250162 & 2002 TY57 & - & - & - & - & - & Phot & Bus-DeMeo & S & VIS & {\cite{2016Icar..268..340C}} \\
\hline \\	\bottomrule
\end{tabular}
