# Supplementary material for: Deficit of primitive compositions in binary asteroids and pairs
Source: arXiv:2302.02668 source file (2023-02-06)
Supplement: Supplementary file 2 [file binpbk_cits.tex]

\begin{tabular}{llrrrrrrrrrr}
	\toprule
	Number & Name & D & $\sigma_D$ & D Ref. & $p_V$ & $\sigma_{p_V}$ & Tax. method & Tax. scheme & Class & Waverange & Tax. Ref. \\
	\midrule
\hline \\30958 & 1994 TV3 & 1.93 & 0.1 & {\cite{2011ApJ...741...68M}} &  0.63 & 0.21  & Phot & Bus-DeMeo & C & VIS & {\cite{2013Icar..226..723D}} \\
33325 & 1998 RH3 & 1.62 & 0.19 & {\cite{2011ApJ...741...68M}} &  0.72 & 0.3  & Phot & Bus-DeMeo & X & VIS & {\cite{2022A&A...658A.109S}} \\
33341 & 1998 WA5 & 2.54 & 0.01 & {\cite{2016AJ....152...63N}} &  0.26 & 0.18  & 0.0 & 0.0 & 0.0 & 0.0 & {\cite{0.0}} \\
58897 & 1998 KZ & - & - & - & - & - & Phot & Bus-DeMeo & X & VIS & {\cite{2013Icar..226..723D}} \\
85563 & 1998 BF7 & - & - & - & - & - & Phot & Bus-DeMeo & X & VIS & {\cite{2013Icar..226..723D}} \\
96334 & 1997 HH3 & - & - & - & - & - & 0.0 & 0.0 & 0.0 & 0.0 & {\cite{0.0}} \\
99263 & 2001 OZ31 & - & - & - & - & - & Phot & Bus-DeMeo & X & VIS & {\cite{2022A&A...658A.109S}} \\
104581 & 2000 GA82 & - & - & - & - & - & Phot & Bus-DeMeo & C & VIS & {\cite{2013Icar..226..723D}} \\
118382 & 1999 JH6 & - & - & - & - & - & Phot & Bus-DeMeo & X & VIS & {\cite{2021A&A...652A..59S}} \\
124122 & 2001 KY2 & - & - & - & - & - & Phot & Bus-DeMeo & X & VIS & {\cite{2013Icar..226..723D}} \\
160609 & 1999 TA35 & - & - & - & - & - & Phot & Bus-DeMeo & X & VIS & {\cite{2013Icar..226..723D}} \\
190622 & 2000 WT49 & - & - & - & - & - & Phot & Bus-DeMeo & X & VIS & {\cite{2021A&A...652A..59S}} \\
\hline \\	\bottomrule
\end{tabular}
