# Supplementary material for: Deficit of primitive compositions in binary asteroids and pairs
Source: arXiv:2302.02668 source file (2023-02-06)
Supplement: Supplementary file 3 [file bins_cits.tex]

\begin{tabular}{llrrrrrrrrrr}
	\toprule
	Number & Name & D & $\sigma_D$ & D Ref. & $p_V$ & $\sigma_{p_V}$ & Tax. method & Tax. scheme & Class & Waverange & Tax. Ref. \\
	\midrule
\hline \\1016 & Anitra & 9.98 & 0.07 & {\cite{2011ApJ...741...68M}} &  0.3 & 0.18  & Spec & Mahlke & S & VISNIR & {\cite{2022A&A...665A..26M}} \\
1798 & Watts & 6.88 & 0.09 & {\cite{2012ApJ...759L...8M}} &  0.24 & 0.19  & Spec & Mahlke & S & VISNIR & {\cite{2022A&A...665A..26M}} \\
2491 & Tvashtri & 3.13 & 0.09 & {\cite{2022PSJ.....3...30M}} &  0.7 & 0.19  & Spec & Mahlke & A & VISNIR & {\cite{2022A&A...665A..26M}} \\
2881 & Meiden & 5.84 & 0.07 & {\cite{2014ApJ...791..121M}} &  0.27 & 0.19  & Spec & Mahlke & S & VISNIR & {\cite{2022A&A...665A..26M}} \\
3122 & Florence & 4.4 & 0.03 & {\cite{2022PSJ.....3...30M}} &  0.26 & 0.18  & Spec & Mahlke & S & VISNIR & {\cite{2022A&A...665A..26M}} \\
3792 & Preston & 5.13 & 0.2 & {\cite{2016AJ....152...63N}} &  0.29 & 0.2  & Spec & Mahlke & S & VISNIR & {\cite{2022A&A...665A..26M}} \\
4435 & Holt & 5.56 & 0.27 & {\cite{2022PSJ.....3...56H}} &  0.26 & 0.21  & Spec & Mahlke & S & VISNIR & {\cite{2022A&A...665A..26M}} \\
4666 & Dietz & 6.73 & 0.4 & {\cite{2016AJ....152...63N}} &  0.25 & 0.22  & Spec & Mahlke & A & VISNIR & {\cite{2022A&A...665A..26M}} \\
7002 & Bronshten & 3.12 & 0.31 & {\cite{2017A&A...603A..55A}} &  0.2 & 0.27  & Spec & Mahlke & S & VISNIR & {\cite{2022A&A...665A..26M}} \\
15745 & Yuliya & 0.77 & 0.15 & {\cite{2010AJ....140..770T}} &  0.32 & 0.44  & Spec & Mahlke & S & VISNIR & {\cite{2022A&A...665A..26M}} \\
190166 & 2005 UP156 & 1.04 & 0.02 & {\cite{2015ApJ...814..117N}} &  0.2 & 0.19  & Spec & Mahlke & S & VISNIR & {\cite{2022A&A...665A..26M}} \\
226514 & 2003 UX34 & - & - & - & - & - & Spec & Mahlke & S & VISNIR & {\cite{2022A&A...665A..26M}} \\
\hline \\	\bottomrule
\end{tabular}
