# Supplementary material for: Deficit of primitive compositions in binary asteroids and pairs
Source: arXiv:2302.02668 source file (2023-02-06)
Supplement: Supplementary file 4 [file binsbk_cits.tex]

\begin{tabular}{llrrrrrrrrrr}
	\toprule
	Number & Name & D & $\sigma_D$ & D Ref. & $p_V$ & $\sigma_{p_V}$ & Tax. method & Tax. scheme & Class & Waverange & Tax. Ref. \\
	\midrule
\hline \\4581 & Asclepius & - & - & - & - & - & Spec & Mahlke & X & VISNIR & {\cite{2022A&A...665A..26M}} \\
33342 & 1998 WT24 & 0.4 & 0.06 & {\cite{2004PhDT.......371D}} &  0.67 & 0.35  & Spec & Mahlke & K & VISNIR & {\cite{2022A&A...665A..26M}} \\
88254 & 2001 FM129 & 0.8 & 0.01 & {\cite{2014ApJ...784..110M}} &  0.22 & 0.19  & Spec & Mahlke & Q & VISNIR & {\cite{2022A&A...665A..26M}} \\
138971 & 2001 CB21 & 0.34 & 0.01 & {\cite{2011PASJ...63.1117U}} &  0.58 & 0.2  & Spec & Mahlke & S & VISNIR & {\cite{2022A&A...665A..26M}} \\
152563 & 1992 BF & 0.37 & 0.1 & {\cite{2012ApJ...760L..12M}} &  0.16 & 0.56  & Spec & Mahlke & K & VISNIR & {\cite{2022A&A...665A..26M}} \\
164202 & 2004 EW & 0.16 & 0.03 & {\cite{2011AJ....141..109M}} &  0.31 & 0.37  & Spec & Mahlke & E & VISNIR & {\cite{2022A&A...665A..26M}} \\
208023 & 1999 AQ10 & 0.15 & 0.04 & {\cite{2016AJ....152..172T}} &  0.5 & 0.56  & Spec & Mahlke & S & VISNIR & {\cite{2022A&A...665A..26M}} \\
281375 & 2008 JV19 & - & - & - & - & - & Spec & Mahlke & X & VISNIR & {\cite{2022A&A...665A..26M}} \\
310442 & 2000 CH59 & - & - & - & - & - & Spec & Mahlke & Q & VISNIR & {\cite{2022A&A...665A..26M}} \\
401885 & 2001 RV17 & - & - & - & - & - & Spec & Mahlke & S & VISNIR & {\cite{2022A&A...665A..26M}} \\
474163 & 1999 SO5 & - & - & - & - & - & Spec & Mahlke & S & VISNIR & {\cite{2022A&A...665A..26M}} \\
518810 & 2010 CF19 & 0.08 & 0.01 & {\cite{2014ApJ...784..110M}} &  0.47 & 0.23  & Spec & Mahlke & S & VISNIR & {\cite{2022A&A...665A..26M}} \\
\hline \\	\bottomrule
\end{tabular}
