# Supplementary material for: Deficit of primitive compositions in binary asteroids and pairs
Source: arXiv:2302.02668 source file (2023-02-06)
Supplement: Supplementary file 5 [file pairp_cits.tex]

\begin{tabular}{llrrrrrrrrrr}
	\toprule
	Number & Name & D & $\sigma_D$ & D Ref. & $p_V$ & $\sigma_{p_V}$ & Tax. method & Tax. scheme & Class & Waverange & Tax. Ref. \\
	\midrule
\hline \\34380 & Pratikvangal & 2.2 & 0.55 & {\cite{2011ApJ...741...68M}} &  0.26 & 0.53  & Phot & Bus-DeMeo & S & VIS & {\cite{2013Icar..226..723D}} \\
38184 & 1999 KF & 2.0 & 0.37 & {\cite{2011ApJ...741...68M}} &  0.31 & 0.41  & Phot & Bus-DeMeo & S & VIS & {\cite{2013Icar..226..723D}} \\
43008 & 1999 UD31 & - & - & - & - & - & Phot & Bus-DeMeo & S & VIS & {\cite{2022A&A...658A.109S}} \\
44620 & 1999 RS43 & - & - & - & - & - & Phot & Bus-DeMeo & S & VIS & {\cite{2022A&A...658A.109S}} \\
48652 & 1995 VB & 2.25 & 0.23 & {\cite{2011ApJ...741...68M}} &  0.23 & 0.27  & Phot & Bus-DeMeo & S & VIS & {\cite{2013Icar..226..723D}} \\
49791 & 1999 XF31 & - & - & - & - & - & Phot & Bus-DeMeo & S & VIS & {\cite{2022A&A...658A.109S}} \\
51609 & 2001 HZ32 & 1.97 & 0.67 & {\cite{2011ApJ...741...68M}} &  0.3 & 0.71  & Phot & Bus-DeMeo & V & VIS & {\cite{2022A&A...658A.109S}} \\
51866 & 2001 PH3 & 3.86 & 0.12 & {\cite{2015ApJ...814..117N}} &  0.25 & 0.19  & Phot & Bus-DeMeo & S & VIS & {\cite{2022A&A...658A.109S}} \\
52478 & 1995 TO & - & - & - & - & - & Phot & Bus & S & VIS & {\cite{2010A&A...510A..43C}} \\
55764 & 1992 DG12 & - & - & - & - & - & Phot & Bus-DeMeo & A & VIS & {\cite{2022A&A...658A.109S}} \\
55913 & 1998 FL12 & - & - & - & - & - & Phot & Bus-DeMeo & X & VIS & {\cite{2022A&A...658A.109S}} \\
56700 & 2000 LL28 & - & - & - & - & - & Phot & Bus-DeMeo & S & VIS & {\cite{2013Icar..226..723D}} \\
\hline \\	\bottomrule
\end{tabular}
