# Supplementary material for: Deficit of primitive compositions in binary asteroids and pairs
Source: arXiv:2302.02668 source file (2023-02-06)
Supplement: Supplementary file 6 [file pairpbk_cits.tex]

\begin{tabular}{llrrrrrrrrrr}
	\toprule
	Number & Name & D & $\sigma_D$ & D Ref. & $p_V$ & $\sigma_{p_V}$ & Tax. method & Tax. scheme & Class & Waverange & Tax. Ref. \\
	\midrule
\hline \\121204 & 1999 OK2 & 1.26 & 0.17 & {\cite{2011ApJ...741...68M}} &  0.6 & 0.32  & Phot & Bus-DeMeo & X & VIS & {\cite{2021A&A...652A..59S}} \\
159931 & 2005 VY5 & - & - & - & - & - & Phot & Bus-DeMeo & X & VIS & {\cite{2013Icar..226..723D}} \\
220878 & 2004 XJ40 & - & - & - & - & - & Phot & Bus-DeMeo & K & VIS & {\cite{2021A&A...652A..59S}} \\
258998 & 2002 TD69 & - & - & - & - & - & Phot & Bus & C & VIS & {\cite{2010A&A...510A..43C}} \\
277930 & 2006 KG118 & - & - & - & - & - & Phot & Bus-DeMeo & S & VIS & {\cite{2022A&A...658A.109S}} \\
311326 & 2005 NE29 & - & - & - & - & - & Phot & Bus-DeMeo & S & VIS & {\cite{2022A&A...658A.109S}} \\
315017 & 2007 BH44 & - & - & - & - & - & Phot & Bus-DeMeo & X & VIS & {\cite{2021A&A...652A..59S}} \\
334028 & 2000 XT37 & - & - & - & - & - & Phot & Bus & C & VIS & {\cite{2010A&A...510A..43C}} \\
348349 & 2005 EQ102 & - & - & - & - & - & Phot & Bus-DeMeo & X & VIS & {\cite{2021A&A...652A..59S}} \\
466986 & 2016 BF39 & - & - & - & - & - & Phot & Bus-DeMeo & S & VIS & {\cite{2022A&A...658A.109S}} \\
485865 & 2012 FL10 & - & - & - & - & - & Phot & Bus-DeMeo & X & VIS & {\cite{2021A&A...652A..59S}} \\
570429 & 2006 RY21 & - & - & - & - & - & Phot & Bus-DeMeo & X & VIS & {\cite{2021A&A...652A..59S}} \\
\hline \\	\bottomrule
\end{tabular}
