# Supplementary material for: Deficit of primitive compositions in binary asteroids and pairs
Source: arXiv:2302.02668 source file (2023-02-06)
Supplement: Supplementary file 7 [file pairs_cits.tex]

\begin{tabular}{llrrrrrrrrrr}
	\toprule
	Number & Name & D & $\sigma_D$ & D Ref. & $p_V$ & $\sigma_{p_V}$ & Tax. method & Tax. scheme & Class & Waverange & Tax. Ref. \\
	\midrule
\hline \\42946 & 1999 TU95 & 4.75 & 0.1 & {\cite{2011ApJ...741...68M}} &  0.2 & 0.19  & Spec & Mahlke & S & VISNIR & {\cite{2022A&A...665A..26M}} \\
52852 & 1998 RB75 & 2.53 & 0.38 & {\cite{2011ApJ...741...68M}} &  0.27 & 0.35  & Spec & Mahlke & V & VISNIR & {\cite{2022A&A...665A..26M}} \\
53537 & Zhangyun & - & - & - & - & - & Spec & Mahlke & S & VISNIR & {\cite{2022A&A...665A..26M}} \\
54041 & 2000 GQ113 & 2.68 & 0.73 & {\cite{2011ApJ...741...68M}} &  0.28 & 0.57  & Spec & Mahlke & V & VISNIR & {\cite{2022A&A...665A..26M}} \\
54827 & Kurpfalz & 2.09 & 0.54 & {\cite{2011ApJ...741...68M}} &  0.24 & 0.55  & Spec & Mahlke & Q & VISNIR & {\cite{2022A&A...665A..26M}} \\
63440 & Rozek & - & - & - & - & - & Spec & Mahlke & C & VISNIR & {\cite{2022A&A...665A..26M}} \\
74096 & 1998 QD15 & - & - & - & - & - & Spec & Mahlke & S & VISNIR & {\cite{2022A&A...665A..26M}} \\
88604 & 2001 QH293 & 5.8 & 0.13 & {\cite{2011ApJ...741...68M}} &  0.2 & 0.19  & Spec & Mahlke & S & VISNIR & {\cite{2022A&A...665A..26M}} \\
92652 & 2000 QX36 & - & - & - & - & - & Spec & Mahlke & S & VISNIR & {\cite{2022A&A...665A..26M}} \\
101703 & 1999 CA150 & - & - & - & - & - & Spec & Mahlke & S & VISNIR & {\cite{2022A&A...665A..26M}} \\
\hline \\	\bottomrule
\end{tabular}
