# Supplementary material for: Deficit of primitive compositions in binary asteroids and pairs
Source: arXiv:2302.02668 source file (2023-02-06)
Supplement: Supplementary file 8 [file pairsbk_cits.tex]

\begin{tabular}{llrrrrrrrrrr}
	\toprule
	Number & Name & D & $\sigma_D$ & D Ref. & $p_V$ & $\sigma_{p_V}$ & Tax. method & Tax. scheme & Class & Waverange & Tax. Ref. \\
	\midrule
\hline \\1920 & Sarmiento & 2.85 & 0.16 & {\cite{2011ApJ...741...68M}} &  0.51 & 0.22  & Spec & Mahlke & E & VISNIR & {\cite{2022A&A...665A..26M}} \\
4736 & Johnwood & 2.72 & 0.07 & {\cite{2022PSJ.....3...30M}} &  0.78 & 0.19  & Spec & Mahlke & E & VISNIR & {\cite{2022A&A...665A..26M}} \\
6461 & Adam & 2.6 & 0.47 & {\cite{2016AJ....152...63N}} &  0.43 & 0.41  & Spec & Mahlke & E & VISNIR & {\cite{2022A&A...665A..26M}} \\
7829 & Jaroff & 2.73 & 0.16 & {\cite{2011ApJ...741...68M}} &  0.44 & 0.22  & Spec & Mahlke & E & VISNIR & {\cite{2022A&A...665A..26M}} \\
15692 & 1984 RA & 1.72 & 0.32 & {\cite{2011ApJ...741...68M}} &  0.58 & 0.41  & Spec & Mahlke & E & VISNIR & {\cite{2022A&A...665A..26M}} \\
16585 & 1992 QR & 2.0 & 0.29 & {\cite{2011ApJ...741...68M}} &  0.57 & 0.35  & Spec & Mahlke & E & VISNIR & {\cite{2022A&A...665A..26M}} \\
20043 & Ellenmacarthur & - & - & - & - & - & Spec & Mahlke & S & VISNIR & {\cite{2022A&A...665A..26M}} \\
25884 & Asai & 1.91 & 0.46 & {\cite{2011ApJ...741...68M}} &  0.6 & 0.52  & Spec & Mahlke & E & VISNIR & {\cite{2022A&A...665A..26M}} \\
53424 & 1999 SC3 & - & - & - & - & - & Spec & Mahlke & S & VISNIR & {\cite{2022A&A...665A..26M}} \\
138970 & 2001 CV19 & 1.09 & 0.11 & {\cite{2017A&A...603A..55A}} &  0.28 & 0.27  & Spec & Mahlke & S & VISNIR & {\cite{2022A&A...665A..26M}} \\
230269 & 2001 XZ6 & - & - & - & - & - & Spec & Mahlke & S & VISNIR & {\cite{2022A&A...665A..26M}} \\
275611 & 1999 XX262 & 1.48 & 0.01 & {\cite{2020PSJ.....1....5M}} &  0.04 & 0.18  & Spec & Mahlke & Ch & VISNIR & {\cite{2022A&A...665A..26M}} \\
\hline \\	\bottomrule
\end{tabular}
